# Supplementary material for: Bagging by Learning to Singulate Layers Using Interactive Perception
Source: arXiv:2303.16898 source file (2023-09-01)
Supplement: Supplementary file 1 [file appendix.tex]

\section{Appendix}

\subsection{Action Primitives Implementation Details}
Here, we describe the implementation details for the action primitives.
\begin{itemize}
    \item For \textbf{Shake}, we set number of repetitions $k_s = 3$, %(for data collection it is a number chosen from range between 2 and 4), 
    amplitude $l = 0.7\pi$ radian ($40.1\degree$), and frequency $f = 0.4$~Hz. 
    \item For \textbf{Fold}, we set $d = 28$~cm. %(The robot is actually instructed to go to fixed (0.42, 0.49, 0.24) and given that the robot usually picks at around y = 0.21, we have a travel distance of 28cm.)
    \item For \textbf{Compress}, we set $k_c = 4$, with a pause of $0.9s$ after every repetition to let the bag settle. The robot grasps the bag with an angle $\alpha = \pi / 7$ radian ($25.7\degree$) with the horizontal plane.  
    \item For \textbf{Flip}, we set the gripper grasping angle $\alpha = 45\degree$.
    \item For \textbf{Dilate}, we restrict the dilation angle $\theta = 0 \degree$ and set distance $d = 12$ cm. Gripper stops when it has moved by $d$ or the torque sensor has reached threshold of $0.05\si{\newton\meter}$.
\end{itemize}

\subsection{Details of Grasp Point Selection}
During data collection, the grasp points for each primitive are sampled as follows:
\begin{itemize}
    \item \textbf{Rotate}: Uniformly on the bag.
    \item \textbf{Shake}: Uniformly from the boundary of the bag.
    \item \textbf{Fold}: Uniformly from the boundary of the bag.
    \item \textbf{Compress}: Uniformly from the bag.
    \item \textbf{Flip}: The left and right endpoints of the bag segmentation along a horizontal line.
    \item \textbf{Recenter}: Center of the bag segmentation. %after a bitwise and operation with the workspace mask.
\end{itemize}

During execution of \bagging, the grasp points for each primitive are sampled as follows:

\textbf{\underline{Stage 1}}: 
\begin{itemize}
    \item \textbf{Shake}: Grasp the center of the handle if at least one handle is visible. Otherwise, sample uniformly from the boundary of the bag.
    \item \textbf{Compress}: The robot grasps the bag with an angle $\alpha = \pi / 7$ radian ($25.7\degree$) with the horizontal plane. The grasp point is the center of the bottom region of the bag, where the bottom is inferred from the rim of the bag using a heuristic: Fit a rectangle to the bag, and find the two corners that are farther from the rim. The center bottom of the bag is then approximated by finding the midpoint of those two farther corners and shrink towards the bag center until the midpoint lies on the bag.
    \item \textbf{Flip}: Same as during data collection.
\end{itemize}

\textbf{\underline{Stage 2}}: 
\begin{itemize}
    \item \textbf{Rotate}: Center of the bag segmentation.
    \item \textbf{Dilate}: The two grippers are oriented towards each other with angle $\alpha = \pi / 3$ radian ($60\degree$) with the horizontal plane and positioned around the center of the bag opening with offset by $0.02$ cm each to avoid collision. The bag opening is approximated using the convex hull of the rim prediction. $\theta$ is set to be $0\degree$, and $d = 10$ cm. Gripper stops when it has moved by $d$ or the torque sensor has reached threshold of $0.02\si{\newton\meter}$.
\end{itemize}

\textbf{\underline{Bag Lifting}}: 
\begin{itemize}
    \item \textbf{Pin-Pull}: The two gripper positions $(x_{pin}, y_{pin})$ and $(x_{pull}, y_{pull})$ are the center of the two predicted handles if the handles are visible and the left and right endpoints of the bag segmentation if the handles are not visible.
\end{itemize}

\subsection{Details of Perception Model}
\begin{figure}[t]
\center
\includegraphics[width=0.23\textwidth]{figures/loss.png}
\includegraphics[width=0.23\textwidth]{figures/iou.png}
\caption{
Learning curve of the perception model (Section~\ref{subsec:training}). \textbf{Left}: Training loss. \textbf{Right}: IOU on the validation set.
}
% \vspace{-5pt}
\label{fig:learning_curve}
\end{figure}

We collected 2,000 paired regular-UV images in total across 4 training bags. To obtain the groundtruth segmentation, we use color thresholding from the UV images and dilate the rim and handle labels to connect regions where the UV paint does not glow strongly and filter noises. We use a 80-20 train/validation split for model training. Figure~\ref{fig:learning_curve} shows the learning curve, including the training loss and validation intersection over union (IOU).

\begin{figure}[t]
\center
\includegraphics[width=0.49\textwidth]{figures/perception_model_example_visualization.png}
\caption{
Examples of the prediction of the perception model on the validation dataset. For each of the three columns, the left ``GT'' are the groundtruth labels, and the right ``Pred'' are the model predictions. Both are overlayed on top of the color images, with green indicating handles and red indicating rim.
}
% \vspace{-5pt}
\label{fig:example_prediction}
\end{figure}

\begin{figure*}[t]
\center
\includegraphics[width=1.00\textwidth]{figures/prediction_metric_pos_neg_examples.png}
\caption{
Positive and negative example predictions of bag segmentation as well as illustrations of the metrics (convex hull and elongation) applied to the predicted rim.
}
% \vspace{-10pt}
\label{fig:metrics_pos_neg_examples}
\end{figure*}

Figure~\ref{fig:metrics_pos_neg_examples} illustrates some positive and negative example predictions of bag segmentation as well as the metrics (convex hull and elongation) applied to the predicted rim. We can see that negative examples are mainly due to wrong predicted rim mask, including both type 1 and type 2 errors. This can lead to the estimated opening through convex hull either too large (including other parts of the bag) or too small (when only part of the true rim is recognized). When the predicted rim is noisy and segmented all over the bag, this can also lead to inaccurate elongation estimate.

\subsection{Experiment Details}
For \textbf{\bagging}, we define $S^{(1)}$ to be the bag size in 2D pixel space divided by the maximum bag size obtained from a flat bag and
we set $S^{(1)} = 0.55$, $A_{CH}^{(1)} = 0.15$, $E_{CH}^{(1)} = 4.5$, $A_{CH}^{(2)} = 0.45$, $E_{CH}^{(2)} = 2.88$.

For \textbf{Baseline 1}, we use the depth image to select the position on the bag with the lowest depth. After placing the first object, we take another depth image and select the position on the bag with the lowest depth as the position to place the second object.

For \textbf{Baseline 2}, we use Sobel filter to find the gradient magnitude of the depth image on the bag. We erode the bag boundaries to avoid placing objects on the boundary of the bag. We then select the position with the largest depth gradient values for placing the first object. We repeat the same procedure for placing the second object.

For \textbf{Baseline 3}, we apply the \textbf{Pin-Pull} primitive to the opening of the bag. In particular, we choose the pin position $(x_{pin}, y_{pin})$ as the center of the rim farther from the bag center, and the pull position $(x_{pull}, y_{pull})$ the midpoint between the center of the rim closer to the bag center and the bag center. The intention is to pin the bottom layer of the bag while pulling the top layer of the bag in order to separate the two layers of the bag and create a sideways-facing opening. The robot then attempts to insert the object from the side, regardless of whether the two layers have been truly separated or not, since the overhead camera cannot tell this.

For \textbf{Baseline 4}, the robot first grasps the two handles, one in each gripper. It then lifts the bag in midair and performs two sequences of dynamic actions. It first shakes the bag in the horizontal left-right direction 2 times. This has the effect of separating the two layers of the rim to prevent them from sticking to each other. The robot then flings the bag vertically 3 times. This action allows the air to come into the bag opening and inflate the bag. Then, the robot’s right gripper releases the handle to grasp the object. Humans inspect the RGBD image after gripper release and manually identify and feed in the opening center to prevent perception errors. Finally, the robot inserts the object at the center of the estimated bag opening while the other gripper still holds the bag.
%It estimates the position of the bag opening while the other gripper still grasps the bag handle. Finally, the robot inserts the object at the center of the estimated bag opening while the other gripper still holds the bag.

For \textbf{AutoBag-D}, this is the same as \bagging but without Stage 2. Regardless of whether the bag opening is large enough after Stage 1, the robot estimates the opening and directly inserts the objects.

\subsection{Failure Modes for \bagging}
Here, we describe the details of the failure cases for \bagging and baselines.

For \bagging, we divide the failure modes into 5 categories. 

(A) is caused by both manipulation and perception challenges during the long sequences of manipulation steps. In particular, during manipulation, the gripper may miss the grasp if the grasp region is too flat on the surface to have enough friction, or the bag may slip out of the gripper during dynamic actions such as \textbf{Shake} and \textbf{Compress}. Additionally, the perception module is not always robust and may sometimes only recognize part of the rim. This leads to the convex hull approximation of the opening to underestimate the true opening and causes the robot to perform more Stage 1 and Stage 2 actions than necessary. For example, after \textbf{Compress} and \textbf{Flip}, even when the bag has a large opening, the robot may fail to recognize the entire rim region, leading to the metrics to not meet the thresholds for Stage 2 and causing the robot to repeat the Stage 1 actions. Another example of unnecessary actions can happen during \textbf{Rotate} and \textbf{Dilate}, where the perception module only recognizes part of the opening, causing the robot to keep rotating and dilating the bag. While this conservatism is not fatal on its own, the increased action steps leads to a larger chance of failure rate due to imperfect manipulation, as the opening can easily close again during manipulation. For example, during \textbf{Dilate}, the friction of the bag with the two grippers may not be the same, causing the bag to slide along with one gripper while the other gripper slips. This moves the bag off the center of the workspace. Also, \textbf{Dilate} is effective only when the two grippers start inside or close to the opening. When the perception module fails to recognize the entire opening, the estimated center of the opening will be inaccurate, causing one gripper to start inside the opening and the other gripper to start far from the opening. When sliding in this asymmetric configuration, the grippers not only fail to enlarge the opening but also tend to compress and realign the separating rim of the bag, making it more difficult for future \textbf{Dilate} actions to enlarge the bag.

(B) is caused by the motion planning of the robot. On one hand, YuMi has a limited workspace and collision-free path planning of the two arms is not always successful, especially around singularities. On the other hand, it is difficult to incorporate the bag as an obstacle for motion planning due to inaccurate depth perception and protruding loop handles. As such, the gripper may occasionally hit the bag before and after each manipulation steps by accident, pushing the bag out of the workspace.

(C) is caused by inaccuracy in the rim prediction. When the perception module’s prediction of the rim has either Type 1 or Type 2 errors, the estimated convex hull will deviate from the true opening. In such cases, some objects may not be placed inside the true opening.

(D) is most often caused by non-ideal grasp positions when lifting the bag. In particular, the bag handles are often occluded by the inserted objects or hidden inside the opening after \textbf{Dilate}. In such cases, the robot simply chooses the left and right endpoints of the bag boundary. However, these grasp points may be near the bottom of the bag and lifting at those positions will make the bag upside down, so objects already inside the bag will fall out again. As the objects can all be contained inside the bag only when both grasp points are near the handles or the rim of the bag, poorly chosen grasp points of at least one gripper will prevent full success. % so the bag is lifted straight upwards

(E) is caused by slipped grasps when the bag contains the inserted objects and has nontrivial weights. This is more due to mechanical limitations of the YuMi robot, it has limited ($500$ g) payload, not-so-strong gripping force, and poorly designed jaw grippers that will slightly tilt and open at the end when a large force is applied at the top of the metal clips to close them.

On the test bag, the perception module is the main bottleneck since it has never seen the bag before, leading to many cases where it only recognizes part but not all of the rim. As such, (A) is the dominant reason for failure.

\subsection{Failure Modes for Baselines}
Next, we describe the failure modes of the baselines.

\textbf{Baseline 1}: It turns out lowest depth is not a good approximation of where the opening of a plastic bag is located. Unlike more structured bags such as paper bags or cloth bags, the opening of a plastic bag is not necessarily associated with small depth values since the layers below the rim can easily fold into the opening. As such, placing the objects at the minimum depth value often fails to place them inside the opening.

\textbf{Baseline 2}: Similar to the failure reasons for \textbf{Baseline 1}, the bag opening is often not associated with large gradients in the depth value. It is also worth pointing out that due to specularity and translucency of the plastic bag material, the depth values are not very accurate. It is difficult to distinguish between the wrinkles and the rim as both may show up as edges in the depth image and the rim may not necessarily have sharper edges or form a closed circle.

\textbf{Baseline 3}: We observe that, unless there is already a large separation between the two layers of the bag (distance-wise) so that the pinning gripper can firmly and precisely press only the bottom layer, pulling the top layer of the bag almost always grasps the two layers together simultaneously and fails to create a sideways opening. As the layer of the plastic bag is quite thin, the pinning hand needs to exert a strong force towards the bottom layer against the table but not touching the upper layer, a stringent initial condition that is almost never satisfied with normal sideways-facing bags.

\textbf{Baseline 4}: Failure cases can be categorized into two main reasons: (1) The fling actions fail to open the bag, and (2) the opening closes and the bag folds on itself after one gripper releases the handle. In particular, (1) is the main reason. For (1), we observe that the fling actions can only open the bag when both grippers grasp one layer of the handles (insert into the ring regions of handles). When a gripper grasps both layers of the handle, it effective clamps the two layers of the bag together, making it difficult for the fling action to inflate the opening. For (2), we observe that even if flinging successfully inflate the bag, the opening closes as soon as one gripper releases the handle to grasp the inserted object. This is because the handle is heavy and when released, it collapses onto the bag, causing the entire bag to fold itself and the opening closes. As such, there is no room for the robot to insert the objects.

\textbf{AutoBag-D}: In Tier 3 configurations, the bag opening is not large enough without dilation leading to failed insertions.
